# Supplementary material for: Trust Regions Sell, But Who's Buying? Overlap Geometry as an Alternative Trust Region for Policy Optimization
Source: arXiv:2602.06627 source file (2026-02-06)
Supplement: Supplementary file 1 [file proof_high_lr.tex]

% ============================================================
%  BC vs KL: high-LR stability + low-LR equivalence (proof sketch)
%  (Drop-in LaTeX for ICML-style appendix / theory section)
% ============================================================

\section{Why BC/Hellinger is more stable at high learning rates, and matches KL at low learning rates}
\label{sec:bc_vs_kl_theory}

\paragraph{Setup.}
Let $q(a|s)=\pi_{\text{old}}(a|s)$ and $p_\theta(a|s)=\pi_\theta(a|s)$ denote the old and new policies.
Fix a state $s$ (we suppress $s$ for readability) and define the (pointwise) log-ratio and ratio
\begin{align}
\Delta(a) \;\triangleq\; \log p_\theta(a) - \log q(a),
\qquad
r(a) \;\triangleq\; \frac{p_\theta(a)}{q(a)} \;=\; e^{\Delta(a)} .
\end{align}
The Bhattacharyya coefficient (BC) and squared Hellinger distance are
\begin{align}
\mathrm{BC}(p_\theta,q) \;\triangleq\; \int \sqrt{p_\theta(a)\,q(a)}\,da
\;=\; \mathbb{E}_{a\sim q}\!\left[\sqrt{r(a)}\right],
\qquad
H^2(p_\theta,q) \;\triangleq\; 1-\mathrm{BC}(p_\theta,q).
\end{align}

% ------------------------------------------------------------
\subsection{Low learning-rate regime: BC behaves like KL (second-order equivalence)}
\label{sec:low_lr_equiv}

\begin{lemma}[BC--KL local quadratic equivalence]
\label{lem:bc_kl_local}
Assume $\|\Delta\|_\infty$ is sufficiently small and $\mathbb{E}_q[\Delta]= -\mathrm{KL}(q\|p_\theta)$ is finite.
Then, to second order,
\begin{align}
1-\mathrm{BC}(p_\theta,q)
\;=\;
\frac{1}{8}\,\mathbb{E}_{q}\!\left[\Delta(a)^2\right]
\;+\; O\!\left(\mathbb{E}_q[|\Delta|^3]\right),
\label{eq:bc_local}
\end{align}
and likewise
\begin{align}
\mathrm{KL}(q\|p_\theta)
\;=\;
\frac{1}{2}\,\mathbb{E}_{q}\!\left[\Delta(a)^2\right]
\;+\; O\!\left(\mathbb{E}_q[|\Delta|^3]\right).
\label{eq:kl_local}
\end{align}
Consequently,
\begin{align}
1-\mathrm{BC}(p_\theta,q)
\;=\;
\frac{1}{4}\,\mathrm{KL}(q\|p_\theta)
\;+\;
O\!\left(\mathbb{E}_q[|\Delta|^3]\right).
\label{eq:bc_kl_relation}
\end{align}
\end{lemma}

\begin{proof}
Using $\sqrt{r}=e^{\Delta/2}$ and Taylor expansion around $\Delta=0$,
\begin{align}
e^{\Delta/2}
= 1 + \frac{\Delta}{2} + \frac{\Delta^2}{8} + O(|\Delta|^3).
\end{align}
Taking expectation under $q$ yields
\begin{align}
\mathrm{BC}(p_\theta,q)
= \mathbb{E}_q[e^{\Delta/2}]
= 1 + \frac{1}{2}\mathbb{E}_q[\Delta] + \frac{1}{8}\mathbb{E}_q[\Delta^2]
+ O(\mathbb{E}_q[|\Delta|^3]).
\end{align}
Since $\mathbb{E}_q[\Delta] = \mathbb{E}_q[\log p_\theta - \log q] = -\mathrm{KL}(q\|p_\theta)$,
we get
\begin{align}
1-\mathrm{BC}(p_\theta,q)
= \frac{1}{2}\mathrm{KL}(q\|p_\theta) - \frac{1}{8}\mathbb{E}_q[\Delta^2]
+ O(\mathbb{E}_q[|\Delta|^3]).
\end{align}
Meanwhile, the standard local expansion of KL around $p_\theta=q$ gives \eqref{eq:kl_local}.
Substituting \eqref{eq:kl_local} into the display above cancels the leading term and yields \eqref{eq:bc_local},
and then \eqref{eq:bc_kl_relation} follows by combining \eqref{eq:bc_local} and \eqref{eq:kl_local}.
\end{proof}

\paragraph{Implication for low LR.}
When learning rates are small, the update keeps $\Delta$ in the local regime, so both regularizers induce
(up to constant factors) the same quadratic constraint on $\Delta$:
\[
\mathrm{KL}(q\|p_\theta) \approx \tfrac{1}{2}\mathbb{E}_q[\Delta^2],
\qquad
1-\mathrm{BC}(p_\theta,q) \approx \tfrac{1}{8}\mathbb{E}_q[\Delta^2].
\]
Thus, with matched coefficients, PPO+KL and PPO+BC behave nearly identically, consistent with the observation
($3120$ vs $3121$ at $3\!\times\!10^{-4}$).

% ------------------------------------------------------------
\subsection{High learning-rate regime: BC controls tails and yields stability}
\label{sec:high_lr_stability}

\paragraph{Core identity.}
Define the deviation variable $Y \triangleq \sqrt{r}-1$ under $a\sim q$.
Then
\begin{align}
\mathbb{E}_q[Y^2]
= \mathbb{E}_q[(\sqrt{r}-1)^2]
= \int q\left(\sqrt{\frac{p_\theta}{q}}-1\right)^2
= \int(\sqrt{p_\theta}-\sqrt{q})^2
= 2\bigl(1-\mathrm{BC}(p_\theta,q)\bigr).
\label{eq:hellinger_second_moment}
\end{align}
So penalizing $1-\mathrm{BC}$ \emph{directly} controls a second moment of $\sqrt{r}$.

\begin{lemma}[Chebyshev-style tail bound for ratio explosions]
\label{lem:tail_bound}
For any $t>1$,
\begin{align}
\Pr_{a\sim q}\!\bigl(r(a)\ge t\bigr)
\;\le\;
\frac{2\bigl(1-\mathrm{BC}(p_\theta,q)\bigr)}{\bigl(\sqrt{t}-1\bigr)^2}.
\label{eq:tail_bound}
\end{align}
\end{lemma}

\begin{proof}
Let $Y=\sqrt{r}-1$ and set $\varepsilon=\sqrt{t}-1>0$. Then
\begin{align}
\Pr(r\ge t) = \Pr(\sqrt{r}-1 \ge \varepsilon) \le \Pr(|Y|\ge \varepsilon)
\le \frac{\mathbb{E}[Y^2]}{\varepsilon^2},
\end{align}
by Chebyshev's inequality. Substitute \eqref{eq:hellinger_second_moment} to obtain \eqref{eq:tail_bound}.
\end{proof}

\paragraph{Why this matters at high LR.}
At high learning rates, policy updates can produce larger $\Delta$ and heavier tails in $r=e^\Delta$.
The policy-gradient estimator typically contains $r$ multiplicatively (even with clipping, many samples sit on the clip boundary),
so its variance depends on tail events such as $r\gg 1$. Lemma~\ref{lem:tail_bound} shows that increasing BC (equivalently decreasing
$1-\mathrm{BC}$) \emph{provably} reduces an upper bound on the probability of such large ratios.
In contrast, a KL penalty primarily constrains the \emph{mean} log-ratio, $\mathbb{E}_q[\log r]= -\mathrm{KL}(q\|p_\theta)$,
and does not directly control $\Pr(r\ge t)$ or second moments of $\sqrt{r}$.

% ------------------------------------------------------------
\subsection{Additional stabilization from bounded log-ratio robustification (implementation-consistent)}
\label{sec:bounded_robustification}

\paragraph{Robustified log-ratio.}
Our implementation uses a saturated log-ratio
\begin{align}
\tilde{\Delta}(a) \;\triangleq\; c\,\tanh\!\Bigl(\frac{\Delta(a)}{c}\Bigr),
\qquad \Rightarrow \qquad
\tilde{\Delta}(a)\in[-c,c],
\end{align}
and defines robust weights
\begin{align}
\tilde{r}(a) \triangleq e^{\tilde{\Delta}(a)} \in [e^{-c},e^{c}],
\qquad
\widetilde{\mathrm{BC}} \triangleq \mathbb{E}_q\!\left[e^{\tilde{\Delta}(a)/2}\right]\in[e^{-c/2},e^{c/2}].
\end{align}
Hence, in the BC-regularized objective, both the policy-gradient multiplier $\tilde{r}$ and the BC contribution
are uniformly bounded, preventing rare large-$|\Delta|$ events from producing unbounded gradient magnitudes.

\begin{proposition}[Uniform boundedness of robust multipliers]
\label{prop:bounded}
For all samples $a$,
\begin{align}
\bigl|\tilde{\Delta}(a)\bigr|\le c
\;\Rightarrow\;
\tilde{r}(a)\le e^c,\quad
e^{\tilde{\Delta}(a)/2}\le e^{c/2},
\end{align}
and therefore any term of the form $\tilde{r}(a)\,A(a)$ in the loss has magnitude bounded by $e^c|A(a)|$.
\end{proposition}

\paragraph{Consequence.}
In the high-LR regime, where $\Delta$ can occasionally be large, this boundedness prevents ``single-sample domination''.
Combined with Lemma~\ref{lem:tail_bound} (tail compression in $r$ via BC/Hellinger geometry),
this explains why PPO+BC remains stable and can keep improving at higher learning rates, matching the empirical result
($3501$ vs $3060$ at $5\!\times\!10^{-4}$), while at lower learning rates the local equivalence in Lemma~\ref{lem:bc_kl_local}
explains near-identical performance ($3121$ vs $3120$ at $3\!\times\!10^{-4}$).

% ------------------------------------------------------------
\subsection{Takeaway (one-line)}
\label{sec:takeaway}
\noindent
\textbf{Low LR:} BC and KL coincide to second order ($1-\mathrm{BC}\approx \tfrac{1}{4}\mathrm{KL}$).
\quad
\textbf{High LR:} BC/Hellinger regularization controls ratio tails via \eqref{eq:tail_bound} and (with saturation) bounds
importance multipliers, yielding lower-variance updates and improved stability.
